# Supplementary material for: SpatialSplat: Efficient Semantic 3D from Sparse Unposed Images
Source: arXiv:2505.23044 source file (2025-10-10)
Supplement: Supplementary file 1 [file X_suppl.tex]

\clearpage
\setcounter{page}{1}
\maketitlesupplementary
\section{Details of Contrastive Loss}
As described in Sec.~\ref{method:Semantic_Radiance_Field}, the complexity of the Contrastive loss scales quadratically with the number of pixels.
Existing per-scene optimization methods address this by randomly selecting a subset of pixels for loss calculation in each iteration.
The number of pixels is typically limited to less than 4096 due to the memory constraints of mainstream GPUs.
However, we find that this strategy yields minimal results in feed-forward 3DGS. 
For a $256 \times 256$ image, fewer than 6$\%$ of the pixels' corresponding Gaussian parameters are updated in each iteration. 
This significantly impacts training efficiency and leads to unsatisfactory performance in our experiments.
To address this, we propose a linear-complexity approach for accurately estimating the contrastive loss, aiming to update all Gaussian parameters within a single iteration.
 
We first consider the similarity loss for primitives belonging to the same instance, corresponding to the first part of right side of Eq.~\ref{loss:constrast}.
Given a set of binary masks $\mathcal{M} = \{ \boldsymbol{M^k} \mid k = 1,2,...,m \}$ extracted from SAM,
We flatten both the rendered instance feature map 
$\boldsymbol{F}_I$ and all masks into
$\boldsymbol{F}_I \in \mathbb{R}^{n\times N}$ and $\boldsymbol{M}^i \in \mathbb{R}^n$, where $n$ represents the total number of pixels.
Based on the masks, we separate the features for each instance, shuffle their order, and obtain a new feature map 
$\boldsymbol{F}_I^{\star}$. 
Note that the inter-instance spacing in $\boldsymbol{F}_I^{\star}$ remains preserved.
We then compute the cosine similarity between the features at the same positions in $\boldsymbol{F}_I$ and $\boldsymbol{F}_I^{\star}$, resulting in a computation with a complexity of $\mathbf{O}(n)$.
Intuitively, instead of calculating the similarity between each primitive and all other primitives within an instance, we compute the similarity between each primitive and a single other primitive in the instance.
This is feasible because primitives within the same instance exhibit highly consistent features.
For the similarity computation between primitives from different instances, as shown in the remaining terms on the right side of Eq.~\ref{loss:constrast}, wwe represent each instance by the average feature of its primitives and compute its similarity with other instances.
This results in a complexity of $\mathbf{O}(m^2)$, which can be ignored as $N \gg m$.
Thus, we successfully estimate Eq.~\ref{loss:constrast} with a complexity of $\mathbf{O}(N)$, ensuring that every primitive participates in the computation and receives updates.
Experimental results demonstrate the high effectiveness of our approach.

\section{More Implementation Details}
For SpatialSplat, we employ the AdamW optimizer, setting the initial learning
rate for the backbone to 2 × 10−5 and other parameters to 2 × 10−4. 
The model is trained using 8 A100-40G GPUs with a total batch size of 128, which takes approximately 2 days to complete.
Techniques such as gradient accumulation and Automatic Mixed Precision (AMP) are applied to increase the effective batch size and reduce memory consumption.
All methods take images at a resolution of $256\times256$ as input.
For feed-forward methods, we follow~\cite{free-spalt} and set the input image distance to 25. 
We select four views between the input images for testing, and no masks are used to fill regions without primitives.

\subsection{Large Spatial Model}
Since Large Spatial Model only provides pretrained weights without code for training from scratch, we directly use the pretrained model for comparison.
To ensure a fair comparison, we use the same training dataset, evaluation scenes, and pretrained 2D model.
As the method predicts Gaussians with scale ambiguity, we use the depth maps provided in the ScanNet dataset to recover the scale.
The optimal scale is computed using the Weiszfeld algorithm, as done in the official implementation.

\subsection{NeRF-DFF}
\label{nerf-dff-appendix}
We convert the test dataset to the COLMAP format as required by NeRF-DFF.
We use five images for training and one for testing.
Each training image is first processed by LSeg to extract a $256 \times 256 \times 512$ feature map, which is then used along with the original RGB image to train a feature field.
The default configuration from the official implementation is used.

\subsection{Feature-3DGS}
We preprocess the dataset as described in Sec.~\ref{nerf-dff-appendix}.
For Feature-3DGS, we use the speed-up model with a compressed feature dimension of 128, as recommended in the paper.
Each scene is trained for 7K iterations.
Additionally, we train several selected scenes for 20K iterations, but the performance shows no significant improvement compared to 7K iterations.

\begin{figure*}[t]
\vspace{0.3cm}
\centering
\begin{minipage}{1\linewidth}
    \centering
        \includegraphics[width=1\linewidth]{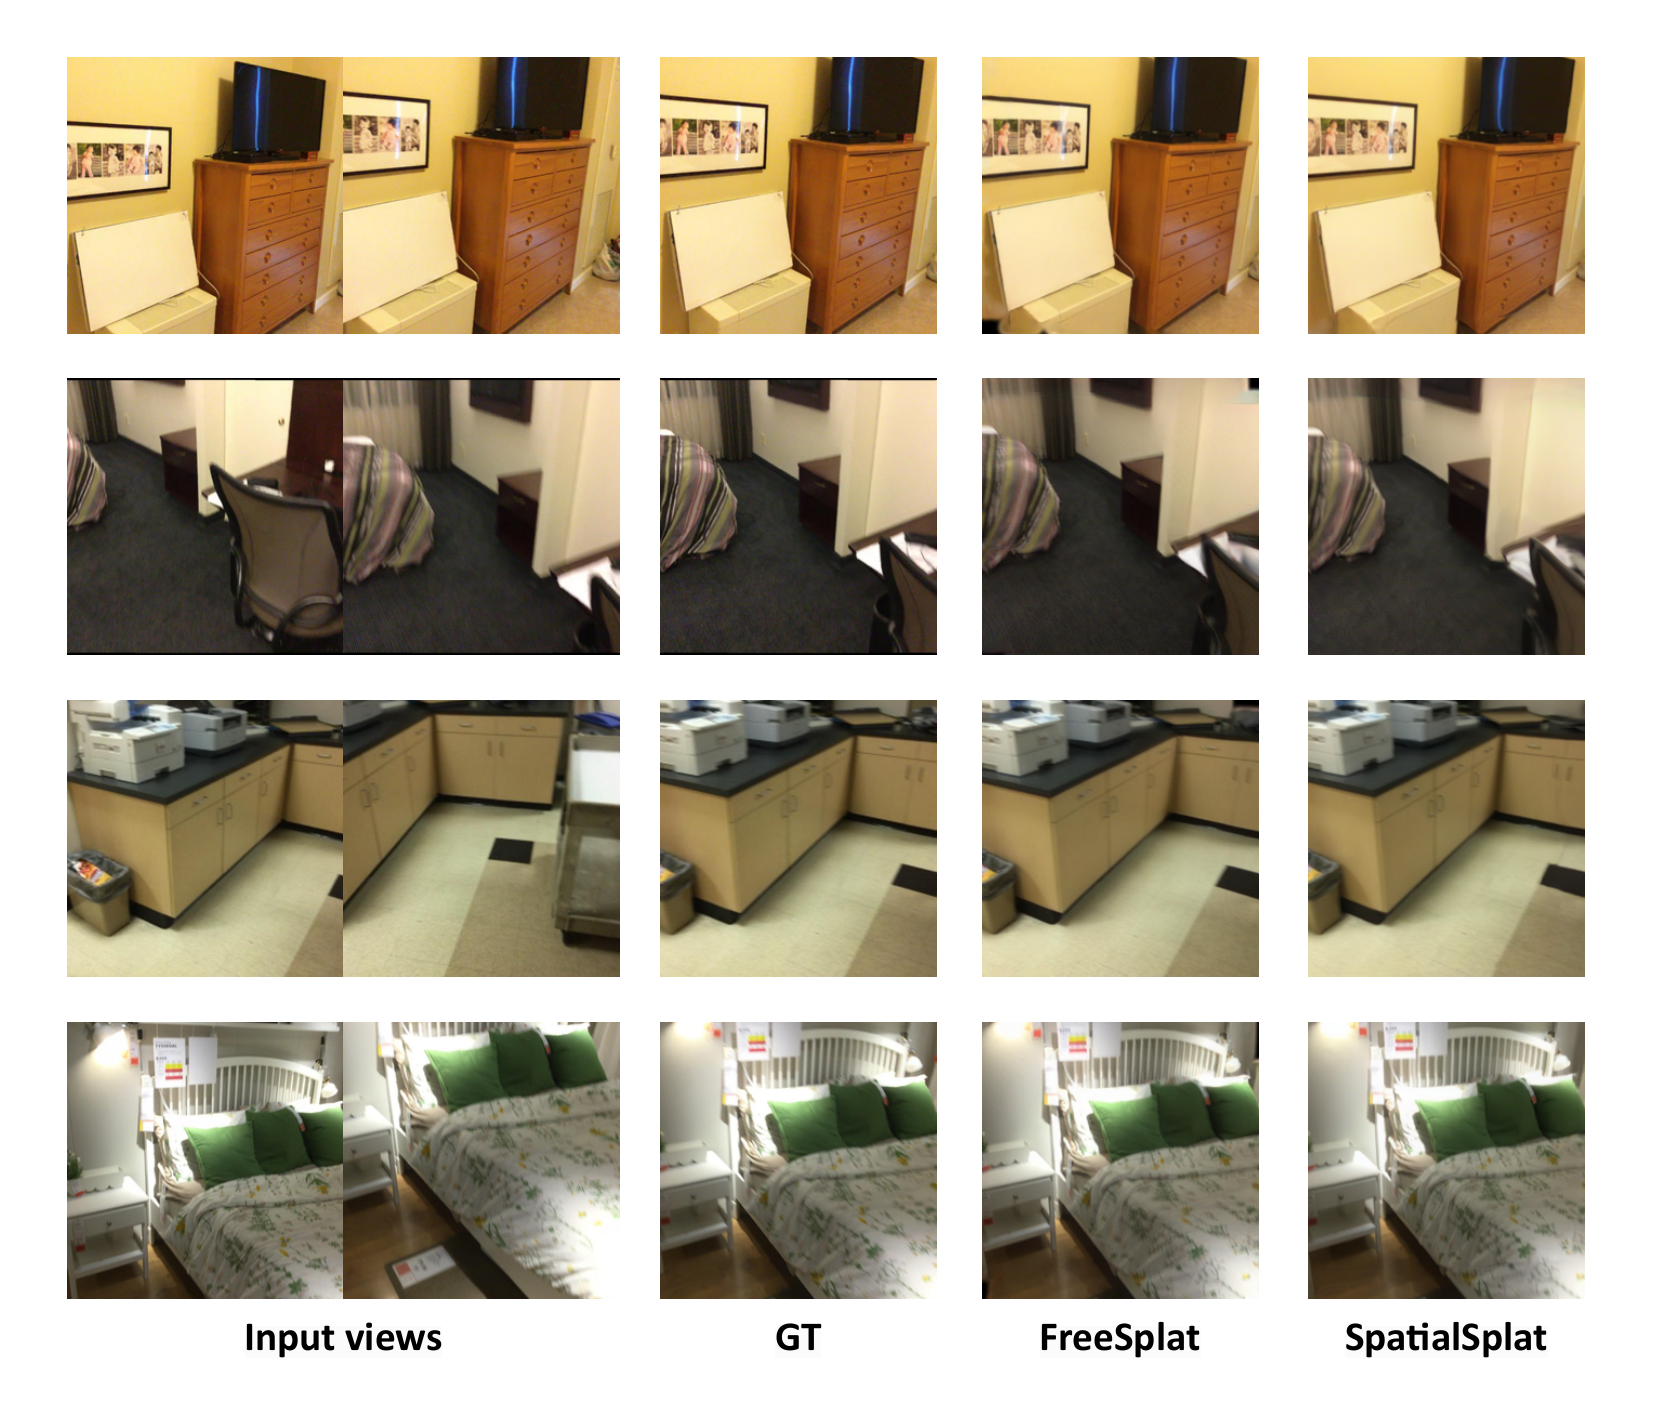}
\end{minipage}
\vspace{-1.5em}
\caption{\textbf{Qualitative comparison results with FreeSplat.}}
% \vspace{-2em}
\end{figure*}

\begin{table*}[t]
\vspace{1em}
    \setlength{\abovecaptionskip}{0em}
    \centering
    \caption{\textbf{Quantitative comparison with FreeSplat.}}
    \label{table:FreeSplat}
    % \resizebox{\linewidth}{!}{
    \begin{tabular}{*{5}{c}}
        \toprule
         Method & PSNR $\uparrow$ & SSIM $\uparrow$ & LPIPS $\downarrow$& Gaussian Num. $\downarrow$\\
        FreeSplat & 26.62 & 0.8485 & 0.1775 & 104K\\
        SpatialSplat & 25.46 & 0.8045 & 0.2046 & 87.7K \\
         \bottomrule
    \end{tabular}
    % }
% \vspace{-2em}
\label{appendix-fig:freesplat}
\end{table*}

\subsection{NoPoSplat}
We retrain NoPoSplat using the code from the official repository.
Notably, we do not apply the inference-time alignment trick proposed in the original paper to improve performance.
This decision is based on our observation that both our method and NoPoSplat achieve good performance on ScanNet without this trick.

\section{More Experimental Analysis}
\subsection{Latency and memory overhead}
The time and memory consumption for each module were measured on an RTX 4090 GPU. Each measurement was averaged over 100 independent runs to ensure reliability.

\begin{table*}[t]
\vspace{1em}
    \setlength{\abovecaptionskip}{0em}
    \centering
    \caption{\textbf{Quantitative results of time and memory consumption.}}
    \label{table:FreeSplat}
    % \resizebox{\linewidth}{!}{
    \begin{tabular}{{l}|{c}{c}{c}{c}{c}{c}}
        \toprule
        Module & 3D Geometry & Semantic Lifting & DPT Heads & Rasterizer & Total \\ 
        \midrule
        Latency & 31ms & 26ms & 17ms & 4ms & 78ms \\
        Memory & 3.2GB & 2.5GB & 0.5GB & 0.2GB & 6.4GB \\ 
         \bottomrule
    \end{tabular}
    % }
% \vspace{-2em}
\end{table*}

% \begin{table}[h]
% \scriptsize
% \vspace{-1em}
%     \setlength{\tabcolsep}{1mm}
%     \setlength{\abovecaptionskip}{0.3em}
%     \centering
%     % \resizebox{\linewidth}{!}{
%     \begin{tabular}{{l}|{c}{c}{c}{c}{c}{c}}
%         \toprule
%         Module & 3D Geometry & Semantic Lifting & DPT Heads & Rasterizer & Total \\ 
%         \midrule
%         Latency & 31ms & 26ms & 17ms & 4ms & 78ms \\
%         Memory & 3.2GB & 2.5GB & 0.5GB & 0.2GB & 6.4GB \\ 
%          \bottomrule
%     \end{tabular}
%     % }
%     \vspace{-1.5em}
% \end{table}

\subsection{More Details of Extension to More Views}
Our SpatialSplat framework can be extended to incorporate additional views.
We designate one view as the reference view, which is processed by Transformer Decoder1 and Heads1 in Fig.\ref{pipeline}.
For other views, we first tokenize them and concatenate all feature tokens before feeding them into the ViT encoder and Transformer Decoder2.
Cross-attention is performed between the reference view tokens and these concatenated tokens.
All other operations remain the same as in the two-view setup.
Gaussian primitives are predicted for each view, and the selective Gaussian mechanism is applied independently to each input view.
The qualitative results of the extension to three views are shown in Fig.\ref{appendix-fig:3view}.

\subsection{Compression With FreeSplat}
FreeSplat is a recent method that employs a feed-forward network to predict 3D Gaussians.
Both our method and FreeSplat recognize that pixel-wise Gaussian prediction is redundant, especially in overlapping areas.
However, there are key differences between SpatialSplat and FreeSplat.
First, FreeSplat is specifically designed for radiance field generation and lacks semantic awareness.
Second, FreeSplat relies on precise camera extrinsics for Gaussian prediction and redundancy identification, making its pipeline fundamentally different from ours.
We primarily compare the two methods in terms of redundancy removal and novel view synthesis.

The performance gap between FreeSplat and our method in novel view synthesis, as shown in Tab.\ref{table:FreeSplat}, is primarily due to the strong geometric prior provided by camera poses.
Similar performance gap between pose-required and pose-free methods have also been observed in\cite{ye2024noposplat,smart2024splatt3r}.
Notably, SpatialSplat uses fewer primitives than FreeSplat, demonstrating that directly identifying redundant primitives from images is feasible.
The qualitative comparison results are presented in Fig.~\ref{appendix-fig:freesplat}.

\section{More Qualitative Results}
We provide additional qualitative results on our proposed dual-field architecture and selective Gaussian mechanism. As shown in Fig.~\ref{appendix-fig:importance-instance}, SpatialSplat effectively identifies redundant Gaussians and generates a consistent instance feature field across multiple scenes.

\vspace{-1.5em}
\begin{figure*}[b]
\vspace{0.3cm}
\centering
\begin{minipage}{1\linewidth}
    \centering
        \includegraphics[width=1\linewidth]{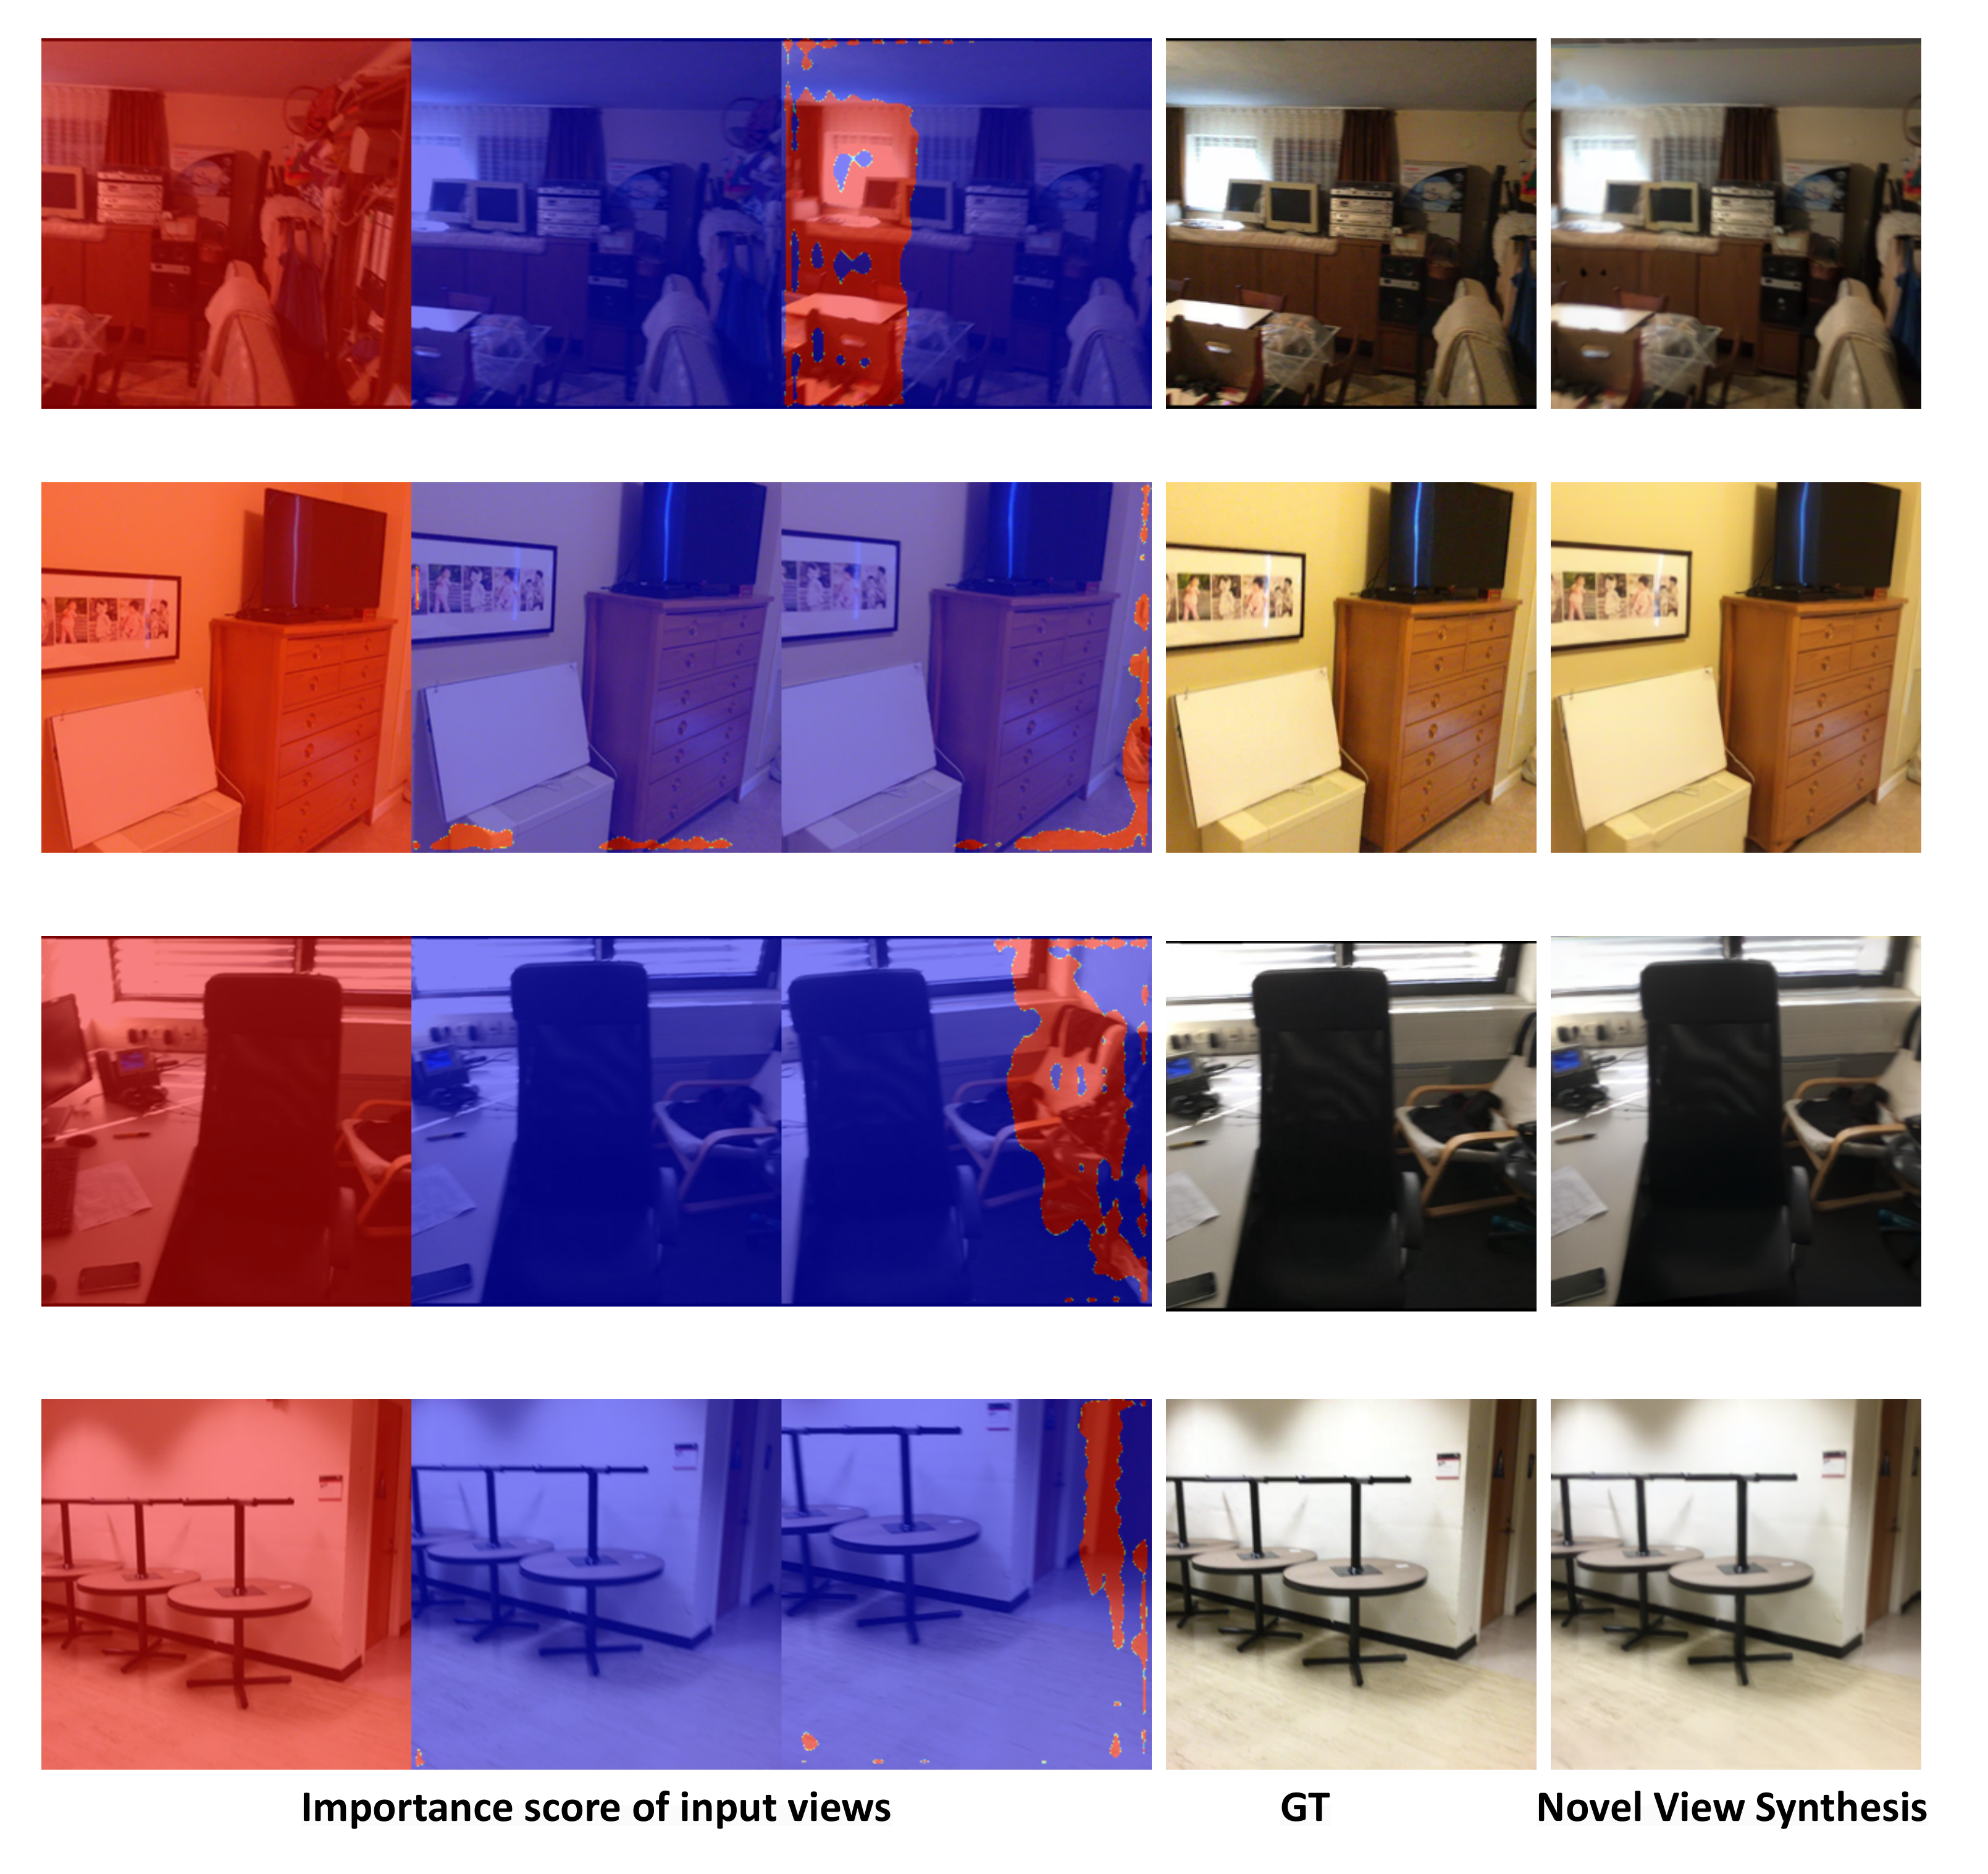}
\end{minipage}
\caption{\textbf{Qualitative results extension to 3 views.}}
\label{appendix-fig:3view}
\vspace{-2em}
\end{figure*}

\begin{figure*}[t]
\vspace{0.3cm}
\centering
\begin{minipage}{1\linewidth}
    \centering
        \includegraphics[width=1\linewidth]{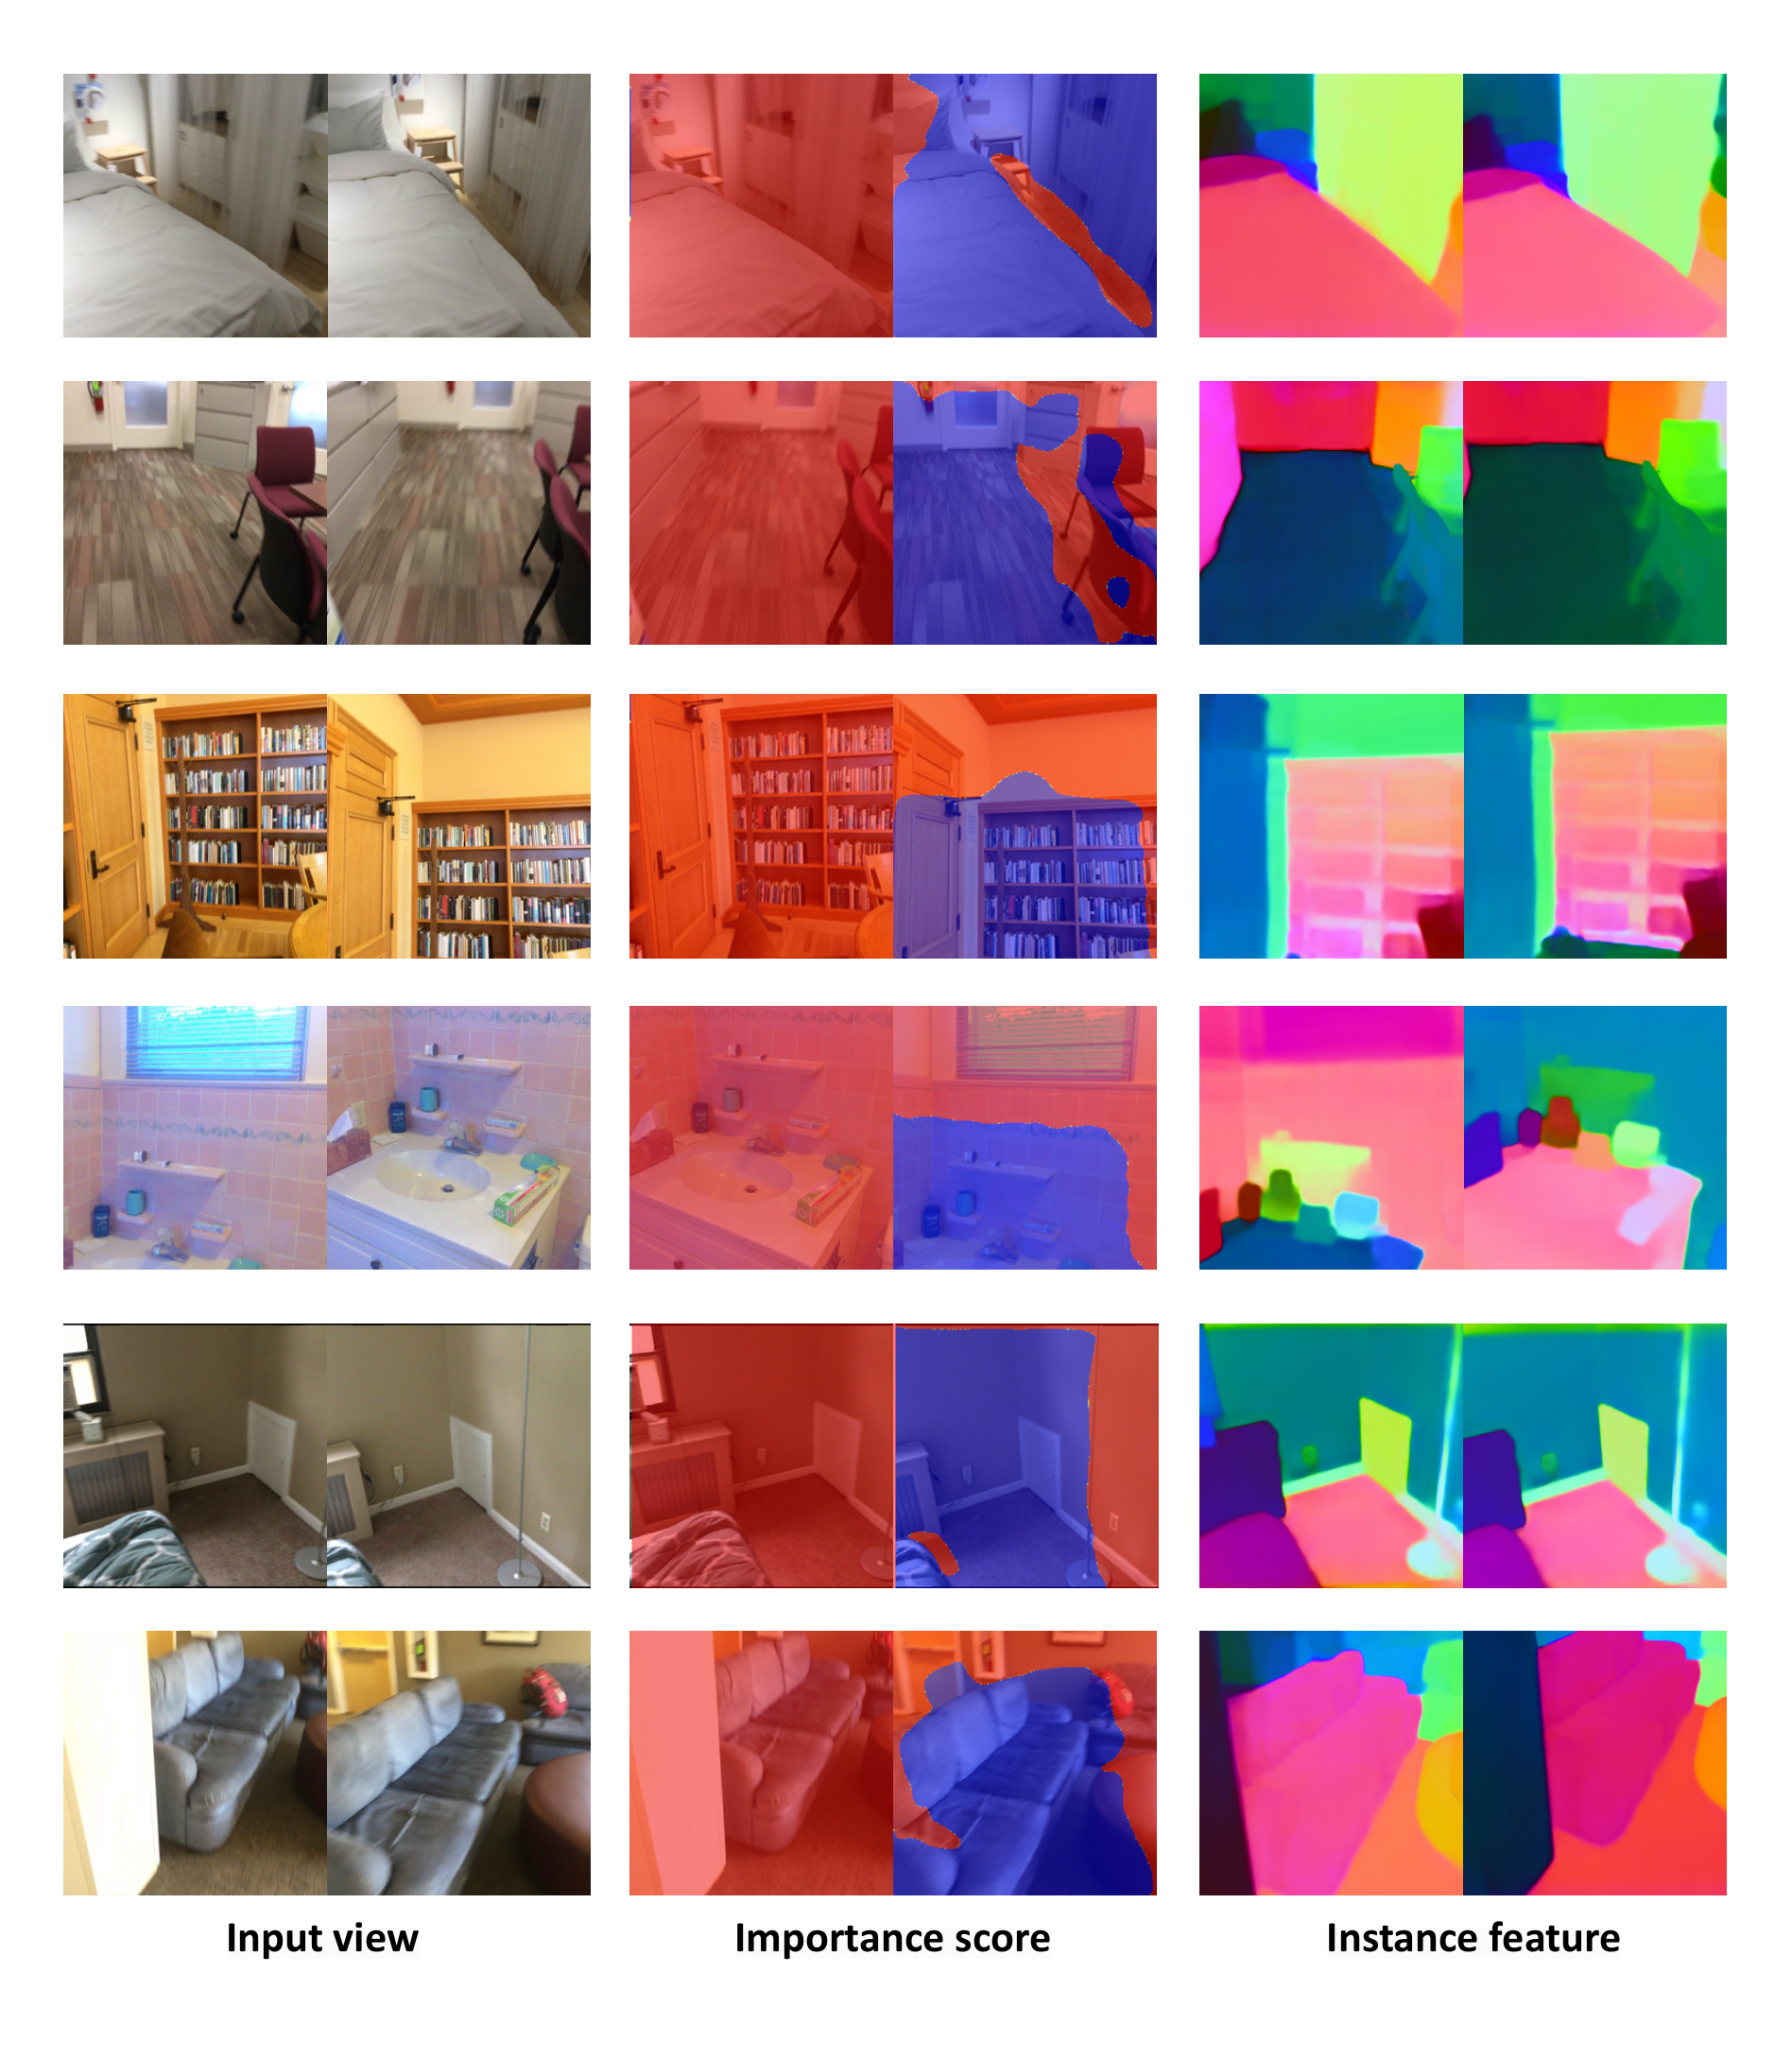}
\end{minipage}
\vspace{-1.5em}
\caption{\textbf{More qualitative results in importance score prediction and instance feature rendering at novel views.}}
\label{appendix-fig:importance-instance}
\vspace{-2em}
\end{figure*}

% \section{Rationale}
% \label{sec:rationale}
% % 
% Having the supplementary compiled together with the main paper means that:
% % 
% \begin{itemize}
% \item The supplementary can back-reference sections of the main paper, for example, we can refer to \cref{sec:intro};
% \item The main paper can forward reference sub-sections within the supplementary explicitly (e.g. referring to a particular experiment); 
% \item When submitted to arXiv, the supplementary will already included at the end of the paper.
% \end{itemize}
% % 
% To split the supplementary pages from the main paper, you can use \href{https://support.apple.com/en-ca/guide/preview/prvw11793/mac#:~:text=Delete%20a%20page%20from%20a,or%20choose%20Edit%20%3E%20Delete).}{Preview (on macOS)}, \href{https://www.adobe.com/acrobat/how-to/delete-pages-from-pdf.html#:~:text=Choose%20%E2%80%9CTools%E2%80%9D%20%3E%20%E2%80%9COrganize,or%20pages%20from%20the%20file.}{Adobe Acrobat} (on all OSs), as well as \href{https://superuser.com/questions/517986/is-it-possible-to-delete-some-pages-of-a-pdf-document}{command line tools}.
